# Supplementary material for: FourLLIE: Boosting Low-Light Image Enhancement by Fourier Frequency Information
Source: arXiv:2308.03033 source file (2023-08-06)
Supplement: Supplementary file 1 [file more_visulization.pdf]

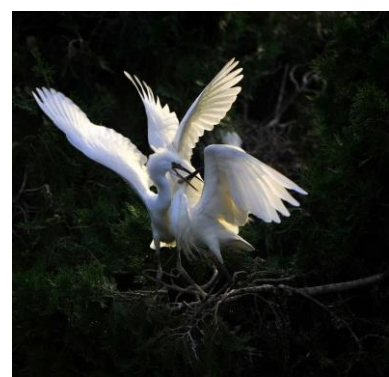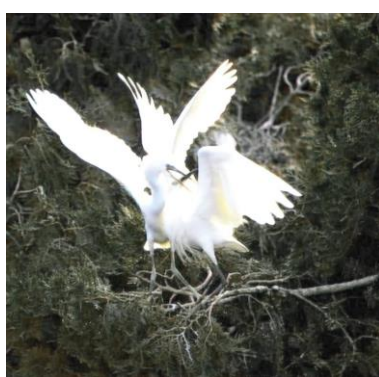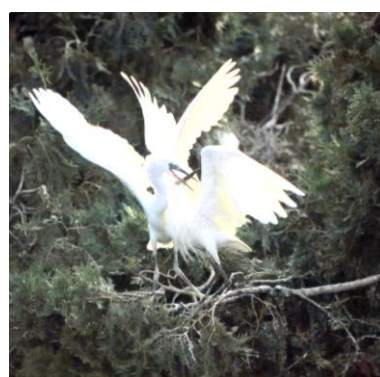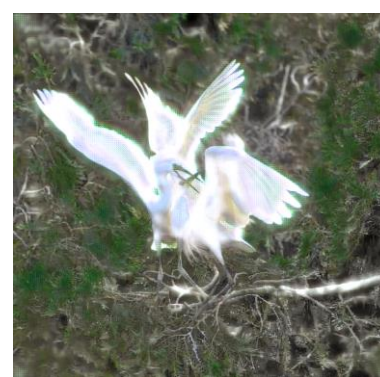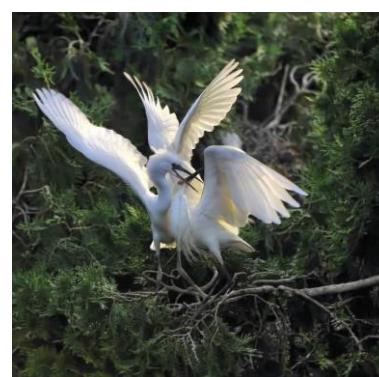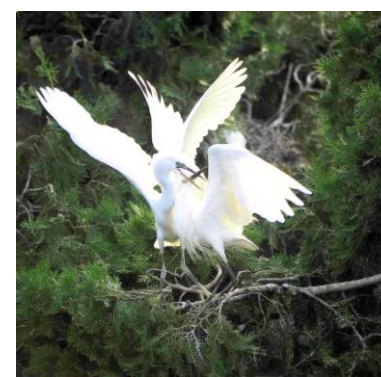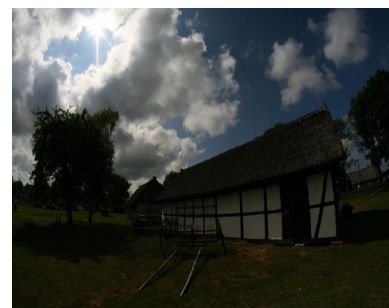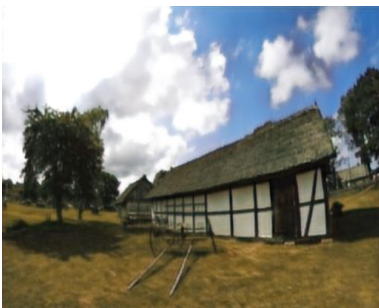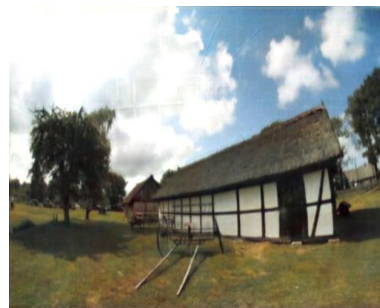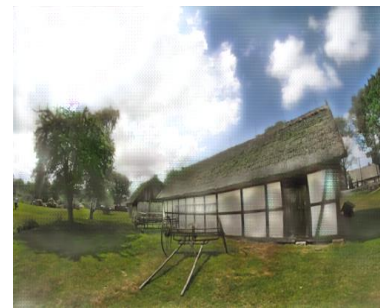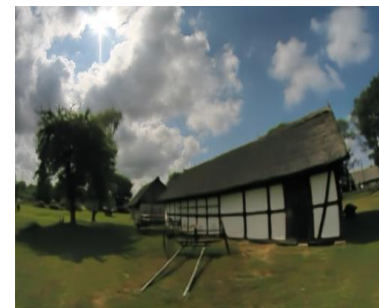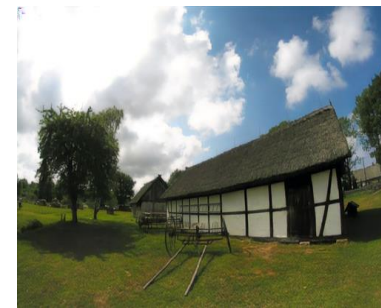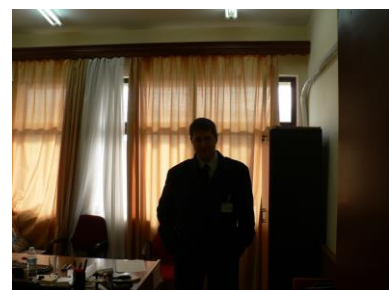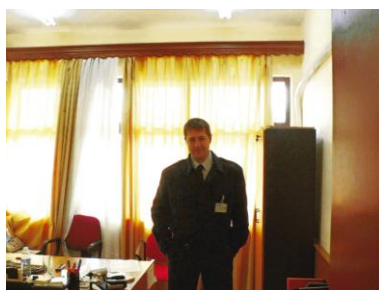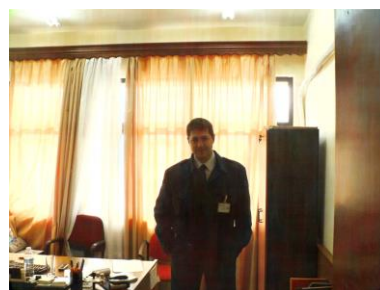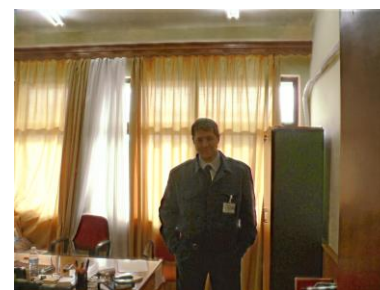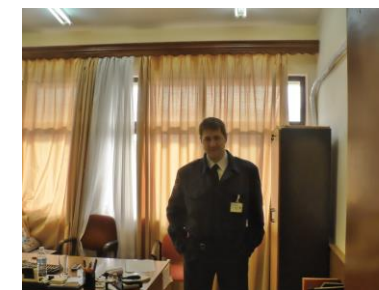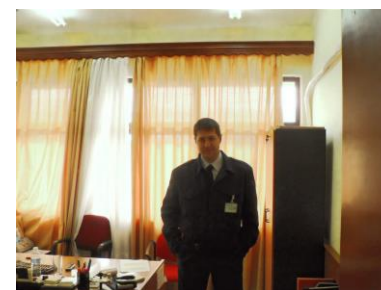

**Input**

**HDMNet**

**FECNet**

**SNR-Aware**

**Bread**

**Ours**



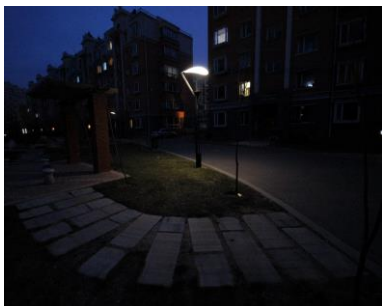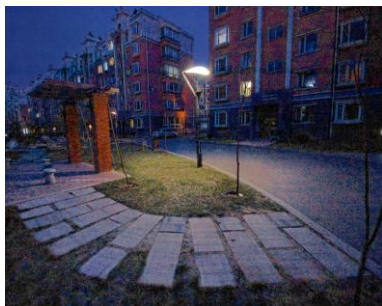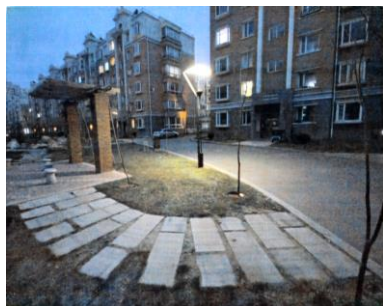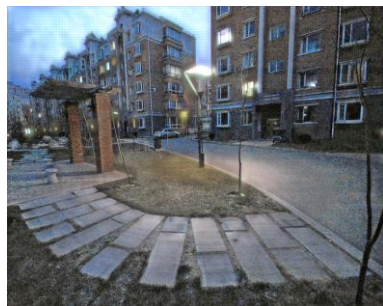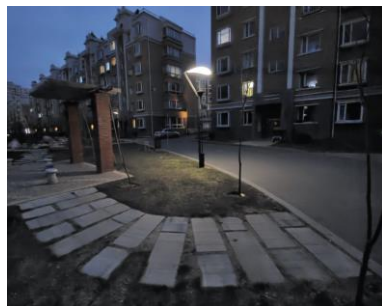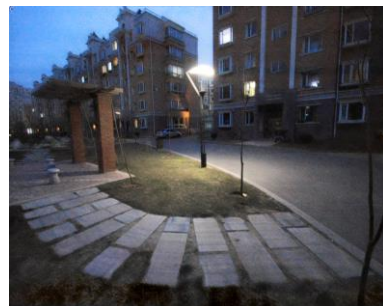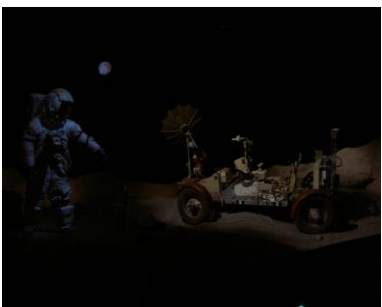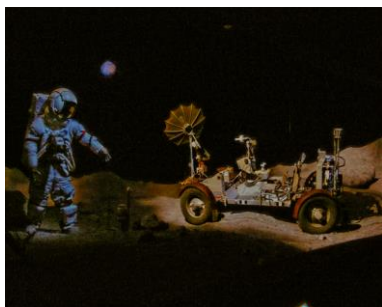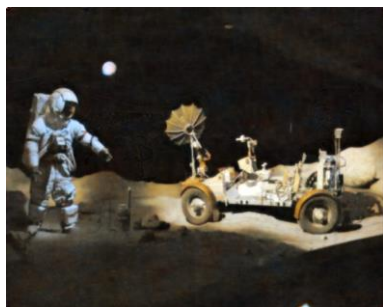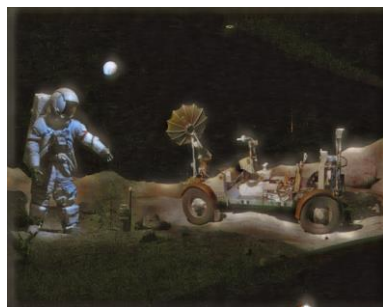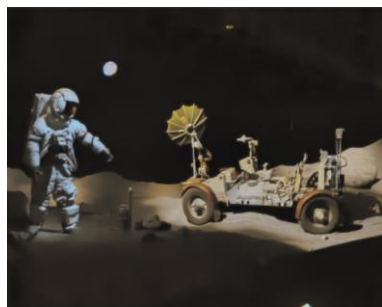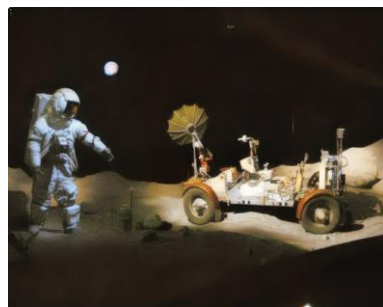

**Input**

**KinD**

**FECNet**

**SNR-Aware**

**Bread**

**Ours**
