# Supplementary material for: FourLLIE: Boosting Low-Light Image Enhancement by Fourier Frequency Information
Source: arXiv:2308.03033 source file (2023-08-06)
Supplement: Supplementary file 2 [file diff_settings.pdf]

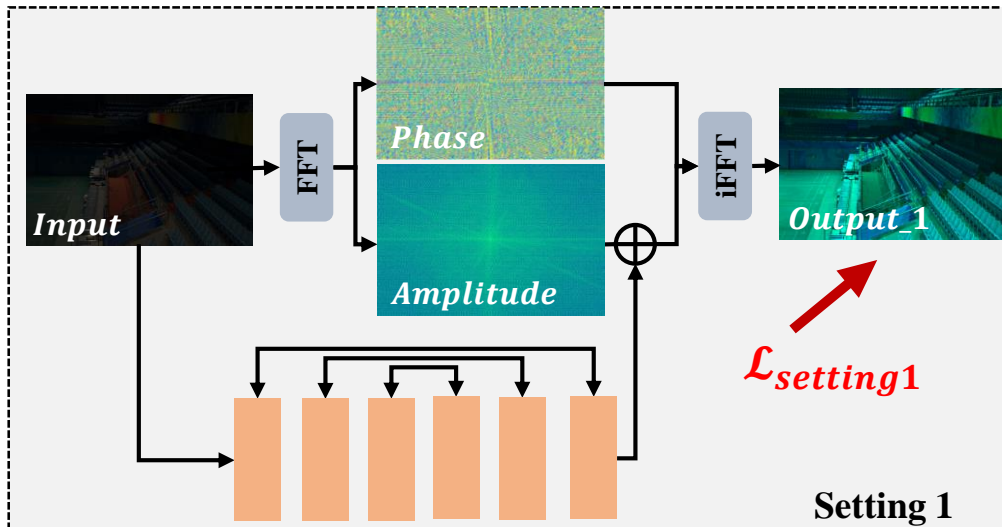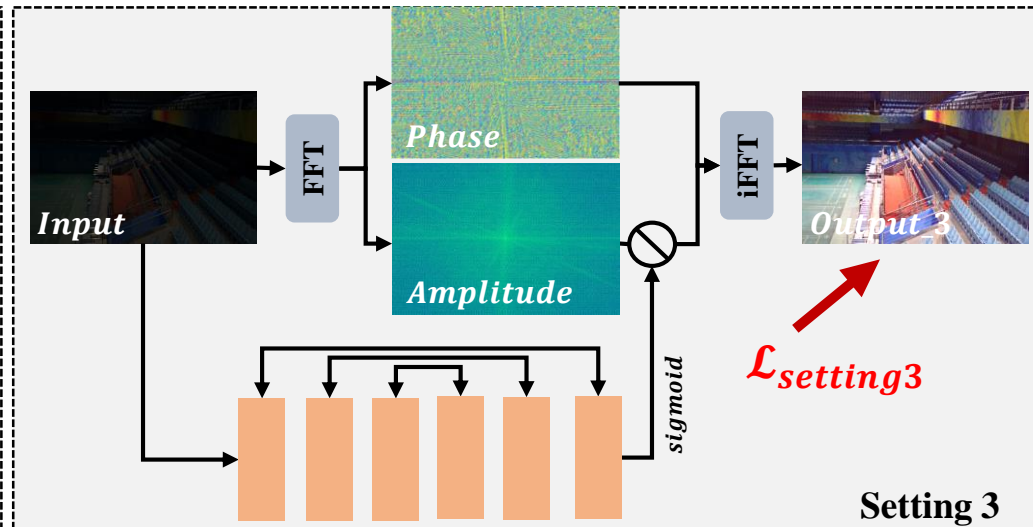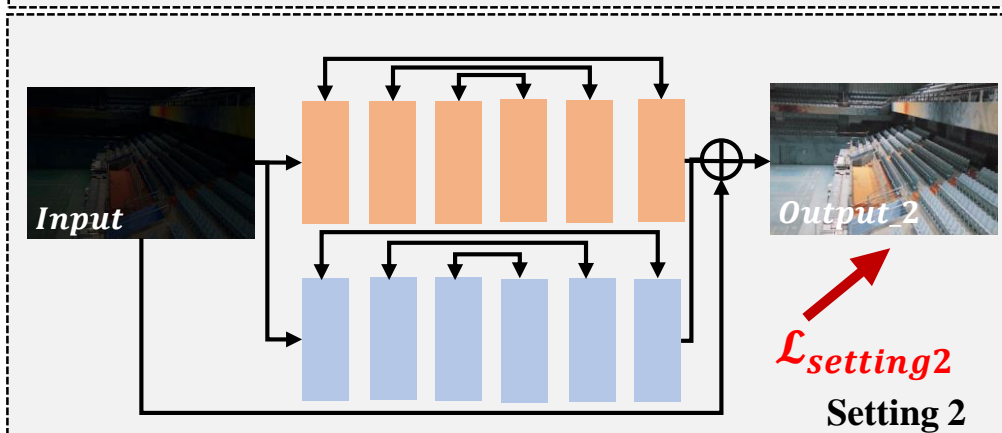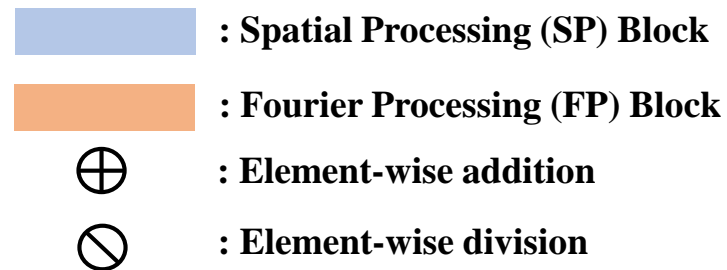

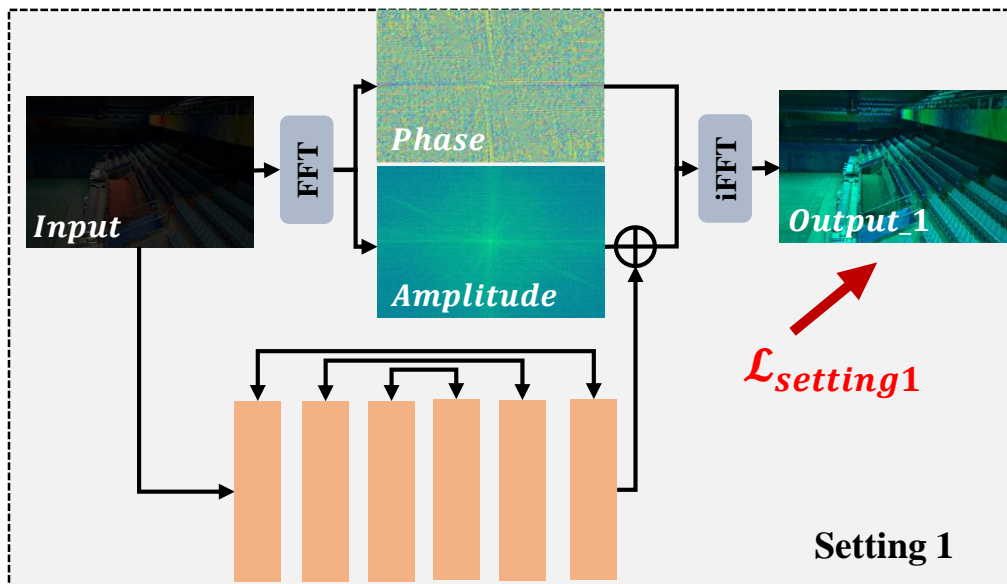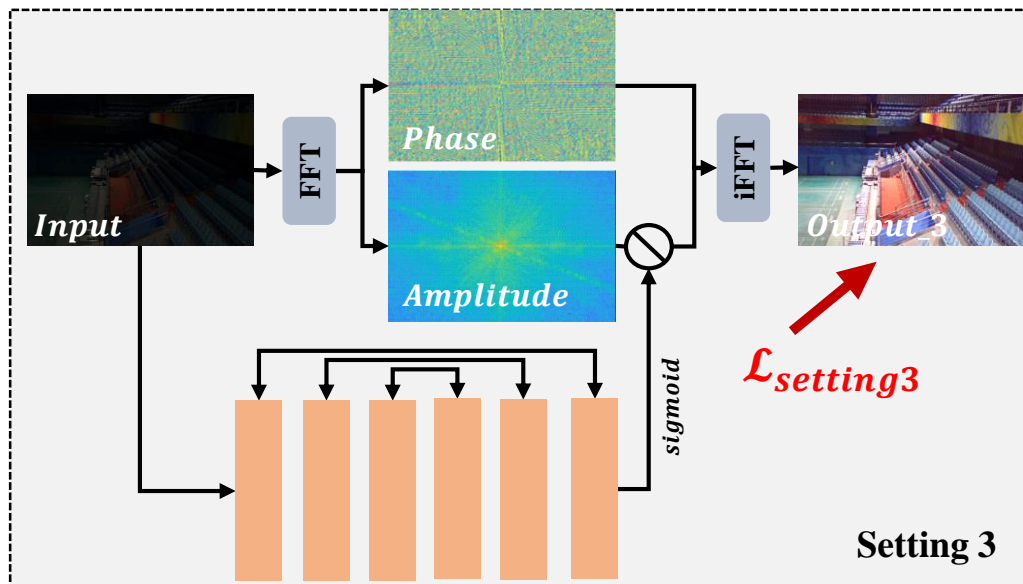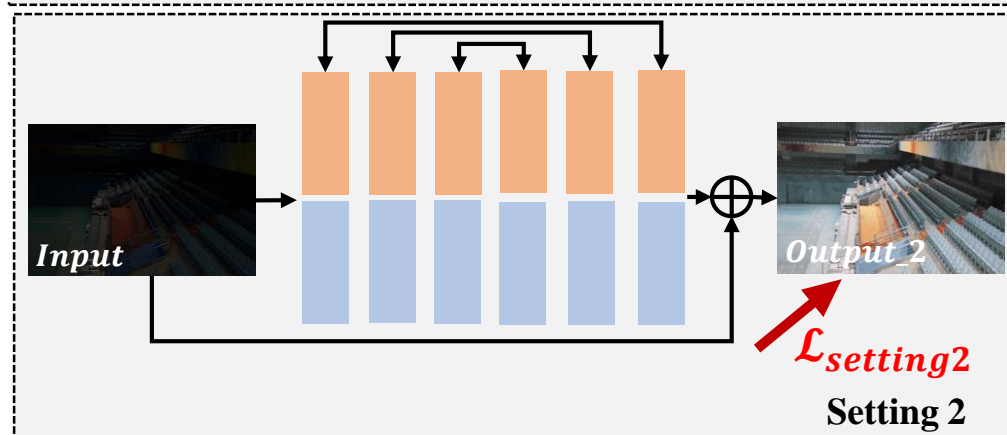

- : Spatial Processing (SP) Block
- : Fourier Processing (FP) Block
- $\oplus$  : Element-wise addition
- $\oslash$  : Element-wise division
